# Supplementary material for: Multicone Diamond Waveguides for Nanoscale Quantum Sensing
Source: arXiv:2306.02966 ancillary file (2023-06-05)
Supplement: Supplementary file 1 [file multicone_supplementary.pdf]

# Supporting Information: Multicone Diamond Waveguides for Nanoscale Quantum Sensing

Tianqi Zhu,† Jan Rhensius,‡ Viraj Damle,‡ Konstantin Herb,† Gabriel Puebla-Hellmann,‡ Christian L. Degen,*,† and Erika Janitz*,†

†*Department of Physics, ETH Zürich, Otto-Stern-Weg 1, 8093 Zürich, Switzerland*

‡*QZabre LLC, Regina-Kägi-Strasse 11, 8050 Zürich, Switzerland*

E-mail: degenc@ethz.ch; ejanitz@phys.ethz.ch

## Wavelength-Dependent Far-Field Emission Intensity

Figure 2b of the main text shows the simulated far-field intensities resulting from NV emission within a 1-μm-tall SC, 5-μm-tall SC, and 5-μm-tall MC. To gain further intuition for the wavelength-dependent device performance, we also plot the far-field intensities for monochromatic emission at 650, 721, and 800 nm (Fig. S1). It is clear that the MC device exhibits superior performance in terms of collimation and directionality at all three wavelengths.

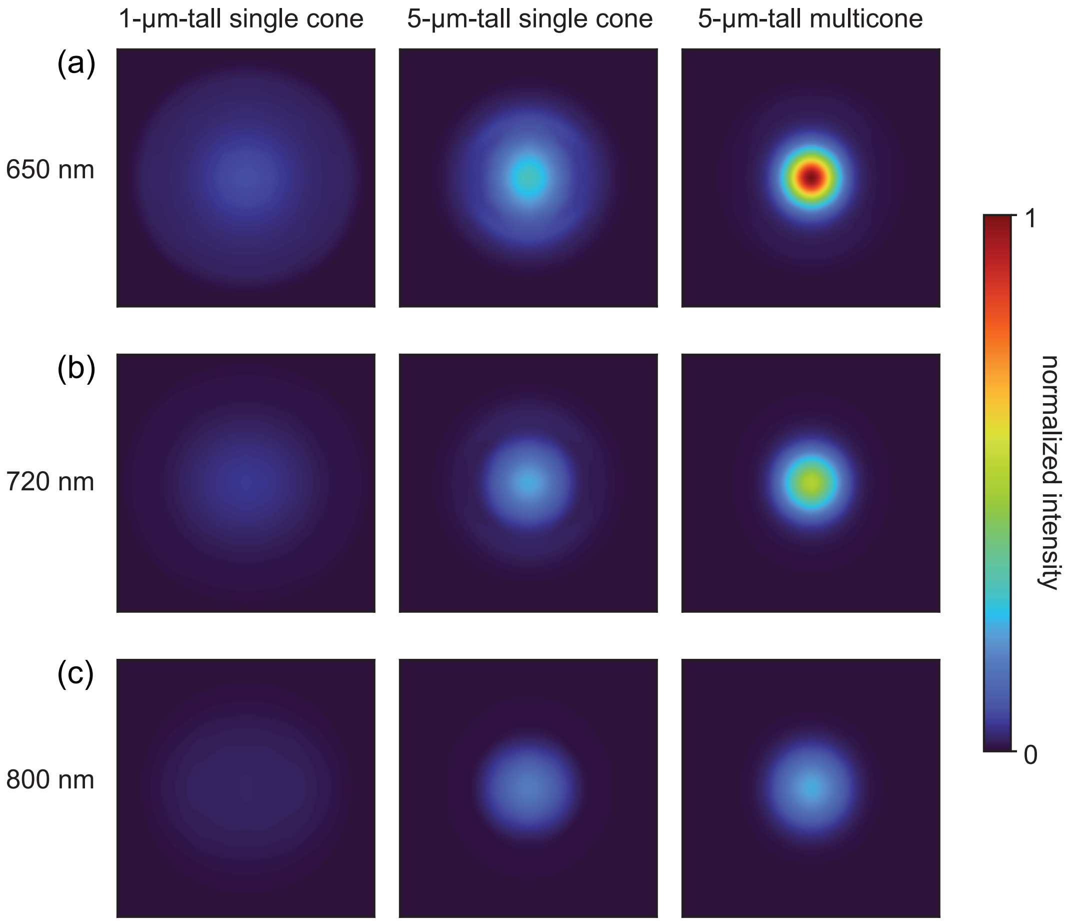


Figure S1: Simulated far-field intensities for 1-μm-tall single-cone, 5-μm-tall single-cone, and 5-μm-tall multicone devices with monochromatic emission at a) 650 nm, b) 721 nm, and c) 800 nm.

# Diamond Fabrication

To ensure consistent material properties, all devices were created from the same electronic-grade diamond plate ((100)-cut, $2 \times 2 \times 0.5$ mm, Element 6), which was subsequently diced into 20-μm-thick membranes (surface roughness $\approx 0.8$ nm-rms, Almax easyLab). An inductively coupled plasma reactive-ion etching (ICP RIE, Oxford Instruments PlasmaPro 100) recipe was used to condition the diamond surface before NV centers were created. This recipe removes $\approx 6$ μm of material to smooth the diamond surface and relieve polishing strain (Tab. S1).

Table S1: Diamond ICP RIE surface conditioning recipe.

| Step | Process | Duration (min) |
|---|---|---|
| 1 | Ar (25 sccm) + $Cl_2$ (40 sccm) | 60 |
| 2 | Ar (25 sccm) + $Cl_2$ (40 sccm) | 5 |
| 3 | $O_2$ (30 sccm) | 10 |
| 4 | 3× repeat steps 2 + 3 | |

Next, NV centers were created using ion implantation (Cutting Edge Ions, 3 keV, $8 \times 10^9$ ions/cm$^3$) and subsequent high-vacuum annealing (880°C for 2 hours, P$< 3 \times 10^{-8}$ mbar).

Pillars were lithographically defined using three layers of electron-beam resist, including a layer of PMGI (SF-8, Kayaku Advanced Materials) followed by 950K PMMA for bilayer liftoff (4.5% in anisole, Allresist), and a final layer of Espacer 300Z to avoid charging (Showa Denko). Following lithography (Raith 150, 20 kV, 20 μm aperture), the resist was developed using a sequence of deionized (DI) water, MIBK, isopropanol, AZ 726 MIF, and DI water. As a mask, a 200-nm-thick layer of aluminum was deposited by electron-beam evaporation (Plassys MEB550S) followed by liftoff in warm DMSO for pillars 1-3. In contrast, a 320-nm-thick aluminum layer was deposited for pillar 4.

Subsequently, pillars 1, 2, and 3 (see Fig. 3 in main text) were defined using an $O_2$-plasma recipe with intermittent $SF_6$ plasma to avoid micromasking (Tabs. S2, S3, and S4). These recipes were terminated once the aluminum mask eroded to a radius of $\approx$ 150 nm (determined using a scanning electron microscope).

Table S2: ICP RIE recipe for pillar 1.

| Step | Process | Duration (min) |
|---|---|---|
| 1 | $SF_6$ (30 sccm) | 0.5 |
| 2 | $SF_6$ (30 sccm) | 0.5 |
| 3 | $O_2$ (50 sccm) | 8 |
| 4 | $SF_6$ (30 sccm) | 0.5 |
| 5 | $SF_6$ (30 sccm) | 0.5 |
| 6 | $O_2$ (50 sccm) | 2 |

Table S3: ICP RIE recipe for pillar 2.

| Step | Process | Duration (min) |
|---|---|---|
| 1 | $SF_6$ (Gas flow: 30 sccm) | 0.5 |
| 2 | $SF_6$ (Gas flow: 30 sccm) | 0.5 |
| 3 | $O_2$ (Gas flow: 50 sccm) | 8 |
| 4 | 2× repeat steps 2 + 3 | |

Table S4: ICP RIE recipe for pillar 3.

| Step | Process | Duration |
|---|---|---|
| 1 | $SF_6$ (30 sccm) | 0.5 |
| 2 | $SF_6$ (30 sccm) | 0.5 |
| 3 | $O2_2$ (50 sccm) | 8 |
| 4 | 4× repeat steps 2 + 3 | |
| 5 | $SF_6$ (30 sccm) | 0.5 |
| 6 | $SF_6$ (30 sccm) | 0.5 |
| 7 | $O_2$ (50 sccm) | 2 |

In contrast, pillar 4 (see Fig. 3 in main text) was first etched with the same recipe as pillars 1-3 until 4.5 μm of material was removed. Next, a mixture of $SF_6$ and $O_2$ was used (Tab. S5) to etch an additional 0.5 μm, resulting in a shallow sidewall angle near the top of the device.

Table S5: ICP RIE recipe for pillar 4.

| Step | Process | Duration (min) |
|---|---|---|
| 1 | $SF_6$ (30 sccm) | 0.5 |
| 2 | $SF_6$ (30 sccm) | 0.5 |
| 3 | $O_2$ (50 sccm) | 10.5 |
| 4 | 4× repeat steps 2 + 3 | |
| 5 | $SF_6$ (10 sccm) + $O_2$ (40 sccm) | 9 |

# Horizontal displacement

We simulate the impact of NV displacement $\delta$ on collection efficiency for pillar 1 (SC) and 4 (MC) devices (Fig. S2). We observe a relatively minor reduction ($< 30\%$ in $\bar{\eta}$) as the NV moves from the center to the edge of the device in both geometries. Consequently, for

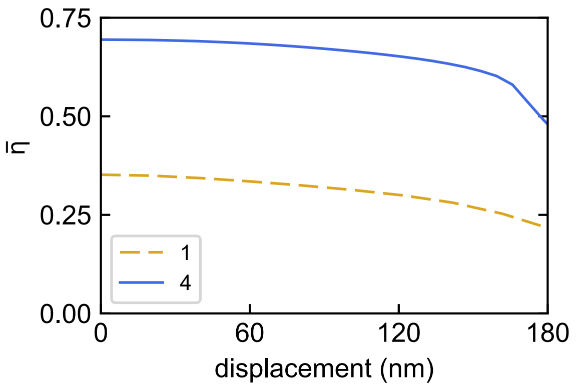


Figure S2: Simulated collection efficiency as a function of NV-center displacement $\delta$ for pillars 1 and 4 ($R_{\text{top}} = 180$ nm for both).

simplicity, we model all emitters as centered within the pillar ($\delta = 0$) at a depth of $d = 5$ nm.

# Single-Photon Emission

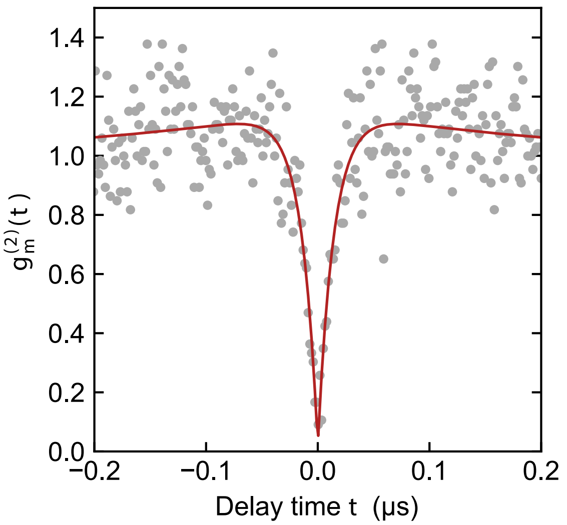


Figure S3: Second-order coherence measurement (grey dots) and fit to Eq. 1 (red line) for a representative pillar 4 device with $g_m^{(2)}(0) = 0.02 \pm 0.06$. Here, we obtain $\rho = 0.99 \pm 0.03$, $\beta = 0.17 \pm 0.03$, $\tau_1 = 14.5 \pm 1.3$ ns, and $\tau_2 = 210 \pm 40$ ns.

We identify pillars containing single NV centers using second-order coherence measurements ($g_m^{(2)}(\tau)$, Fig. S3) measured with a time-correlated single-photon-counting system

(TCSPC, PicoQuant Picoharp 300). These data are fit assuming a Poissonian background parameterized by $\rho = S/(S+B)$, where $S$ is the signal from the NV center and $B$ is the background,[1] yielding

$$g_m^{(2)}(t) = g^{(2)}(t)\rho^2 + 1 - \rho^2, \tag{1}$$

where

$$g^{(2)}(t) = 1 - (1+\beta)e^{-|t|/\tau_1} + \beta e^{-|t|/\tau_2}. \tag{2}$$

Here, $\beta$, $\tau_1$, and $\tau_2$ are fit parameters related to the excitation and decay rates.[1] Single photon emission is unequivocally demonstrated for $g_m^{(2)}(0) < 0.5$; consequently, we select emitters where the sum of the average and standard deviation does not exceed this value.

# Rabi Measurement

We estimate the optical contrast between spin states for a representative pillar 4 device by performing power-dependent Rabi measurements (Fig. S4). Specifically, we fit the first fringe of the oscillation to

$$R(t) = \frac{C\,e^{-t/\tau}}{2}\cos(2\pi f t + \psi) + d, \tag{3}$$

where $C$ is the spin contrast, $\tau$ is the contrast decay constant, $f$ is the Rabi frequency, $\psi$ is a phase offset, and $d$ is the measurement offset.

We observed instability in the laser output power at low power settings ($P_{\mathrm{set}} \leq 1$ mW); consequently, we label each measurement with the programmed power and integrate the photon counts per measurement $\alpha_0$ explicitly in calculating the spin-readout SNR (details in main text).

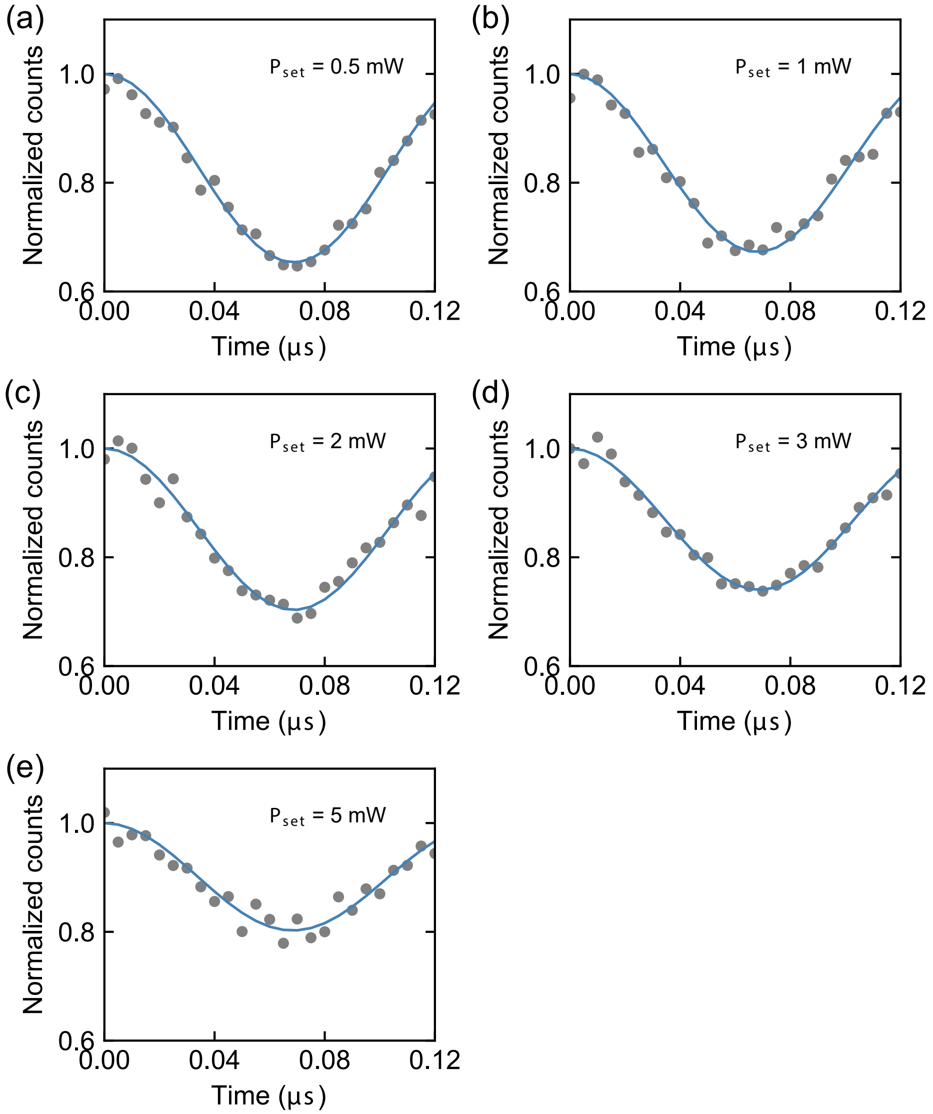


Figure S4: Rabi oscillation measurements (grey dots) at different laser powers for a representative pillar 4 device. Fits to Eq. 3 yield contrast values of a) $C = 34.7 \pm 0.9\%$, b) $C = 32.8 \pm 1.1\%$, c) $C = 29.7 \pm 1.0\%$, d) $C = 26.0 \pm 0.7\%$, and e) $C = 20.1 \pm 1.0\%$.

## References


(1) Brouri, R.; Beveratos, A.; Poizat, J.-P.; Grangier, P. Photon Antibunching in the Fluorescence of Individual Color Centers in Diamond. *Opt. Lett.* **2000**, *25*, 1294–1296.
